# Supplementary material for: Factorization and Normalization, Essentially
Source: arXiv:1908.11289 source file (2019-11-27)
Supplement: Supplementary file 1 [file NO99_-_Appendix.tex]

% !TEX root = main.tex
\section{Proof Appendix}

\begin{lemma}[Substitutivity of $\partobvind n$] %\ref{p:tobv-subs-ind-par}
if $\tm \partobvind n \tm'$ and $\tmtwo \partobvind m \tmtwo'$ where $\tmtwo$ is a value,  then $\tm \isub\var\tmtwo \partobvindlong {n + \sizep{\tm'}\var\cdot m} \tm' \isub\var{\tmtwo'}$.
\end{lemma}

\begin{proof}
	By induction on the definition of $\tm \partobvind{n} \tm'$. Cases:
Cases:
	\begin{enumerate}
	\item \emph{Variable}, \ie $\tm = \var \partobvind{0} \var = \tm'$. Then, $\sizep{\tm'}\var = 1$ and $\tm\isub{\var}{\tmtwo} = \tmtwo \partobvind{m} \tmtwo' = \tm'\isub{\var}{\tmtwo'}$, where $m = 0 + \sizep{\tm'}{\var} \cdot m$.
	\item \emph{Abstraction}, \ie $\tm = \la{\vartwo}{\tmthree} \partobvind{n} \la{\vartwo}{\tmthree'} = \tm'$ because $\tmthree \partobvind{n} \tmthree'$; we can suppose without loss of generality that $\vartwo \notin \fv{\tmtwo} \cup \{\var\} \supseteq \fv{\tmtwo'} \cup \{\var\}$, hence $\sizep{\tmthree'}{\var} = \sizep{\tm'}{\var}$ and $\tm\isub{\var}{\tmtwo} = \la{\vartwo}(\tmthree\isub{\var}{\tmtwo})$ and $\tm'\isub{\var}{\tmtwo'} = \la{\vartwo}(\tmthree'\isub{\var}{\tmtwo'})$.
	By \ih, $\tmthree\isub{\var}{\tmtwo} \partobvindlong{n +  \sizep{\tmthree'}{\var} \cdot m} \tmthree'\isub{\var}{\tmtwo'}$, thus
	\begin{align*}
	\AxiomC{$\tmthree\isub{\var}{\tmtwo} \partobvindlong{n +  \sizep{\tmthree'}{\var} \cdot m} \tmthree'\isub{\var}{\tmtwo'}$}
	%%\RightLabel{$\parRew{\l}$}
	\UnaryInfC{$\tm\isub{\var}{\tmtwo} = \la {\vartwo}\tmthree\isub{\var}{\tmtwo} \partobvindlong{n +  \sizep{\tm'}{\var} \cdot m} \la{\vartwo}\tmthree'\isub{\var}{\tmtwo'} = \tm'\isub{\var}{\tmtwo'}$}
	\DisplayProof\,.
	\end{align*}		
	\item \emph{Application}, \ie $\tm = {\tmthree}\tmfour \partobvind{n_1 + n_2} {\tmthree'}\tmfour' = \tm'$ because $\tmthree \partobvind{n_1} \tmthree'$ and $\tmfour \partobvind{n_2} \tmfour'$.
	By \ih, $\tmthree\isub{\var}{\tmtwo} \partobvindlong{n_1 +  \sizep{\tmthree'}{\var} \cdot m} \tmthree'\isub{\var}{\tmtwo'}$ and $\tmfour\isub{\var}{\tmtwo} \partobvindlong{n_2 +  \sizep{\tmfour'}{\var} \cdot m} \tmfour'\isub{\var}{\tmtwo'}$, hence
	\begin{align*}
	\AxiomC{$\tmthree\isub{\var}{\tmtwo} \partobvindlong{n_1 +  \sizep{\tmthree'}{\var} \cdot m} \tmthree'\isub{\var}{\tmtwo'}$}
	\AxiomC{$\tmfour\isub{\var}{\tmtwo} \partobvindlong{n_2 +  \sizep{\tmfour'}{\var} \cdot m} \tmfour'\isub{\var}{\tmtwo'}$}
	%%\RightLabel{$\parRew{\l}$}
	\BinaryInfC{$\tm\isub{\var}{\tmtwo} = \tmthree\isub{\var}{\tmtwo} \tmfour\isub{\var}{\tmtwo} \partobvindlong{n +  \sizep{\tm'}{\var} \cdot m} \tmthree'\isub{\var}{\tmtwo'} \tmfour'\isub{\var}{\tmtwo'} = \tm'\isub{\var}{\tmtwo'}$}
	\DisplayProof
	\end{align*}
	where $\sizep{\tm'}{\var} = \sizep{\tmthree'}{\var} + \sizep{\tmfour'}{\var}$ and $n = n_1 + n_2$.
	
	\item \emph{$\betav$ step}:
	\[\AxiomC{$\tmthree \partobvind {n_1} \tmthree'$}
	\AxiomC{$\tmfour$ is a value}
	\AxiomC{$\tmfour \partobvind {n_2} \tmfour'$}		
	\TrinaryInfC{$\tm = (\la\vartwo \tmthree)\tmfour \partobvind{n} \tmthree'\isub \vartwo {\tmfour'} = \tm'$}
	\DisplayProof\]
	where $n = n_1 + \sizep{\tmthree'}{\var} \cdot n_2 +1$.
	We can assume without loss of generality that $\vartwo \notin \fv{\tmtwo} \cup \{\var\} \supseteq \fv{\tmtwo'} \cup \{\var\}$;
	hence, $\sizep{\tm'}{\var} = \sizep{\tmthree'}{\var} + \sizep{\tmthree'}{\vartwo}\sizep{\tmfour'}{\var} $ and $\tm\isub{\var}{\tmfour} = (\la{\vartwo}{\tmthree}\isub{\var}{\tmtwo})\tmfour\isub{\var}{\tmtwo}$ and $\tm'\isub{\var}{\tmfour'} = {\tmthree'}\isub{\vartwo}{\tmfour'}\isub{\var}{\tmtwo'} = \tmthree'\isub{\vartwo}{\tmtwo'}\isub{\var}{\tmfour'\isub{\vartwo}{\tmtwo'}}$.
	By \ih, $\tmthree\isub{\var}{\tmtwo} \partobvindlong{n_1 + m \cdot \sizep{\tmthree'}{\var}} \tmthree'\isub{\var}{\tmtwo'}$ and $\tmfour\isub{\var}{\tmtwo} \partobvindlong{n_2 + m \cdot \sizep{\tmfour'}{\var}} \tmfour'\isub{\var}{\tmtwo'}$.
	Therefore, since $\tmfour\isub{\var}{\tmtwo}$ is a value,
	\[\AxiomC{$\tmthree\isub{\var}{\tmtwo} \partobvindlong{n_1 + m \cdot \sizep{\tmthree'}{\var}} \tmthree'\isub{\var}{\tmtwo'}$}
	\AxiomC{$\tmfour\isub{\var}{\tmfour} \partobvindlong{n_2 + m \cdot \sizep{\tmfour'}{\var}} \tmfour'\isub{\var}{\tmtwo'}$}		
	\BinaryInfC{$\tm \isub{\var}{\tmtwo} = (\la\vartwo \tmthree)\tmfour \partobvindlong{n_1 + m \cdot \sizep{\tmthree'}{\var} + (n_2 + m \cdot \sizep{\tmfour'}{\var})\sizep{\tmthree'}{\vartwo} + 1} \tmthree'\isub \vartwo {\tmfour'} = \tm'\isub{\var}{\tmtwo'}$}
	\DisplayProof\]
	where $n_1 + m \cdot \sizep{\tmthree'}{\var} + (n_2 + m \cdot \sizep{\tmfour'}{\var})\sizep{\tmthree'}{\vartwo} + 1 = n + m(\sizep{\tmthree'}{\var} + \sizep{\tmthree'}{\vartwo}\cdot \sizep{\tmfour'}{\var}) = n + m \cdot \sizep{\tm'}{\var}$.
	\qedhere
\end{enumerate}

\end{proof}
