# Supplementary material for: Factorization and Normalization, Essentially
Source: arXiv:1908.11289 source file (2019-11-27)
Supplement: Supplementary file 2 [file toappendix.tex]

\gettoappendix {prop:splitting}
\gettoappendix {prop:completeness}
\gettoappendix {prop:perp}
\gettoappendix {prop:i-e-merge}
